# Supplementary material for: Observation of Electronic Raman Scattering in Metallic Carbon Nanotubes
Source: arXiv:1110.4356 source file (2011-10-19)
Supplement: Supplementary file 1 [file supplementary_110727.pdf]

## SUPPLEMENTARY MATERIAL

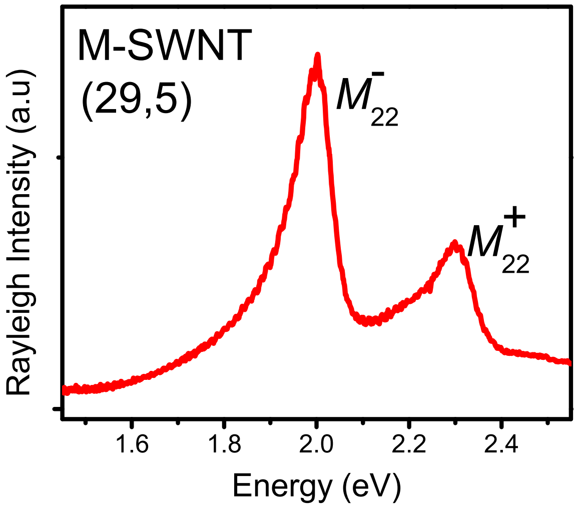


Fig. S 1: The Rayleigh spectrum of the structure-assigned (29,5) $M-$SWNT in Fig. 2(b). The (29,5) $M-$SWNT has a similar diameter but of smaller chiral angle than the (23,14) $M-$SWNT from Fig. 2(a), as indicated by the larger splitting of the $M_{22}^{+}$ and $M_{22}^{-}$ peaks [1].

### Sample preparation

Long aligned carbon nanotubes are grown across the trenches as well as on Si/$SiO_2$ substrates by chemical vapor deposition. The growth is performed at 950°C, using an $FeCl_3$ emulsion as the catalyst and ethanol as the carbon feedstock. To fabricate the trenches, we begin with a 500 $\mu$m thick Si wafer that is coated with a 50nm thick layer of $Si_xN_{1-x}$ deposited by low pressure chemical vapor deposition. Using optical lithography followed by reactive ion etching (RIE), the trench pattern is transfered to the $Si_xN_{1-x}$ layer, on the backside of the wafer, which acts as an etch mask for the Si. A KOH solution is used to wet etch all the way through the Si substrate, resulting in $15 - 50$ $\mu m$ features on the front side of the wafer. The remaining $Si_xN_{1-x}$ mask is etched off and the sample is then annealed in air in order to grow a thin $SiO_2$ layer. Long aligned carbon nanotubes are grown across the trenches by chemical vapor deposition. The growth is performed at 950°C, using an $FeCl_3$ emulsion as the catalyst and ethanol as the carbon feedstock.

**Rayleigh and Raman measurements**

Rayleigh scattering measurements were performed using a white light supercontinuum laser source, as described in [2, 3]. Two achromatic objective lenses oriented at a 90° angle to each other were used to focus the white light spectrum onto the nanotube and to collect the scattered photons, which were then dispersed onto a charged-coupled device array by a single-pass optical spectrometer. The raw Rayleigh spectra were corrected for the supercontinuum spectrum and for the $\omega^3$ systematic dependence of the scattering cross-section expected for an infinite cylinder [4].

Tunable excitation Raman measurements were subsequently carried out using Nd:YAG, Dye (Rhodamine 6G), and Ti:Sapphire lasers, with home-built broadband and high-resolution spectrometers. The Raman experiments were performed at a laser power below 0.6 mW with the beam focused down to a spot size of $\sim 1\mu m$ using a NA=0.75 microscope objective. All spectra have been corrected for detector dark current. All measurements were performed in ambient air at room temperature.

**Structure assignment**

Following Rayleigh measurements, candidate chiral $M-$SWNTs were unambiguously identified through the existence of a broadened, and mildly asymmetric profile in their Raman G-mode spectra [4, 5] (Fig. 1(a), as opposed to $S-$SWNTs, which consistently display narrow ($\sim 5-10$ cm$^{-1}$ FWHM) Lorentzian G-mode features (Fig. 1(b)) [4, 6]. For the nanotubes shown in Figs. 1(a) and (b), the radial breathing mode (RBM) frequencies of $\sim 100$ cm$^{-1}$ (Fig. 1(a)) and 115 cm$^{-1}$ (Fig. 1(b)) suggest diameters of $2.5-2.8$ nm, and $2.3-2.4$ nm, respectively [5, 6].

For the $M-$SWNT, the two Rayleigh peaks (Fig. 1(c) correspond to energies of the second optical transition split by the trigonal warping effect [2, 5] ($M_{22}^{-} = 2.08$ eV, $M_{22}^{+} = 2.19$ eV), while in the case of the $S-$SWNT, the two peaks in Fig. 1(d) correspond to the third and fourth optical transitions with $S_{33} = 1.66$ eV and $S_{44} = 1.84$ eV. A clear exciton-phonon sideband is visible at $\approx 200$ meV above the $S_{44}$ transition, confirming that the nanotube in Fig. 1(d) is an $S-$SWNT [4]. Such sidebands are not apparent for the second-order transitions ($M_{22}$) in large diameter $M-$SWNT [4, 7].

Comparing the energies of the Rayleigh peaks and the RBM frequencies of the nanotubes in Fig. 1 with available data on structurally characterized SWNTs [2, 6], we tentatively assign them to a (23,14) $M-$SWNT and a (25,8) $S-$SWNT, respectively.

**Electrochemical gating**

The electrolyte was prepared by making a 1:2 mixture of $LiClO_4$ and polyethylene oxide in methanol. The working electrode (of the electrochemical cell) consisted of the SWNTs grown on a Si/$SiO_2$ substrate, contacted by an evaporated layer of 5nm of Cr and 30nm of Au. A drop of electrolyte is applied to the sample and is then contacted with a Ag reference electrode and a Pt counter electrode. The gate potential $V_g$ refers to the potential of the reference electrode with respect to the working electrode (the nanotube sample). $E_{\mathrm{F}}$ is scaled linearly to $V_g$ using a ratio of 0.2 eV/V. This gating efficiency is determined as in [8] whereby the $V_g$ range within which the LO phonon is broadened is set equal to the LO phonon energy of 0.2 eV. The Raman spectra are obtained by exciting the nanotubes through the transparent electrolyte using a laser photon energy of 2.33 eV. A background Raman spectrum of the electrolyte and the Si substrate is collected in the immediate vicinity of the nanotube and subtracted from its spectrum. The $M-$SWNT in Fig. 3 has an RBM frequency of $\sim 240$ cm$^{-1}$.

**Determining the electrochemical gating efficency using the LO phonon linewidth:**

In $M-$SWNTs the higher and lower frequency components of the G-band ($G^+$ and $G^-$) [9] are associated with the transverse optical (TO) and longitudinal optical (LO) phonon modes, respectively. The LO mode is known to be broadened and downshifted because of its interaction with low lying e-h pairs [5, 8, 10, 11]. Therefore, the quenching of the ERS feature, brought about by shifting the Fermi level, is also accompanied by the narrowing and hardening of the LO phonon component ($G^-$) of the G-band feature. The fact that the LO linewidth is broadened within the window $|2E_{\mathrm{F}}| < \hbar\omega_{LO}$ allows us to scale the gate voltage $V_g$ to the Fermi energy axis.

For each value of $V_g$, we fit the Raman spectra from the electrochemical gating experiment described in Fig. 3. The ERS feature and the $G^+$ feature are fit to Lorentzian curves. The

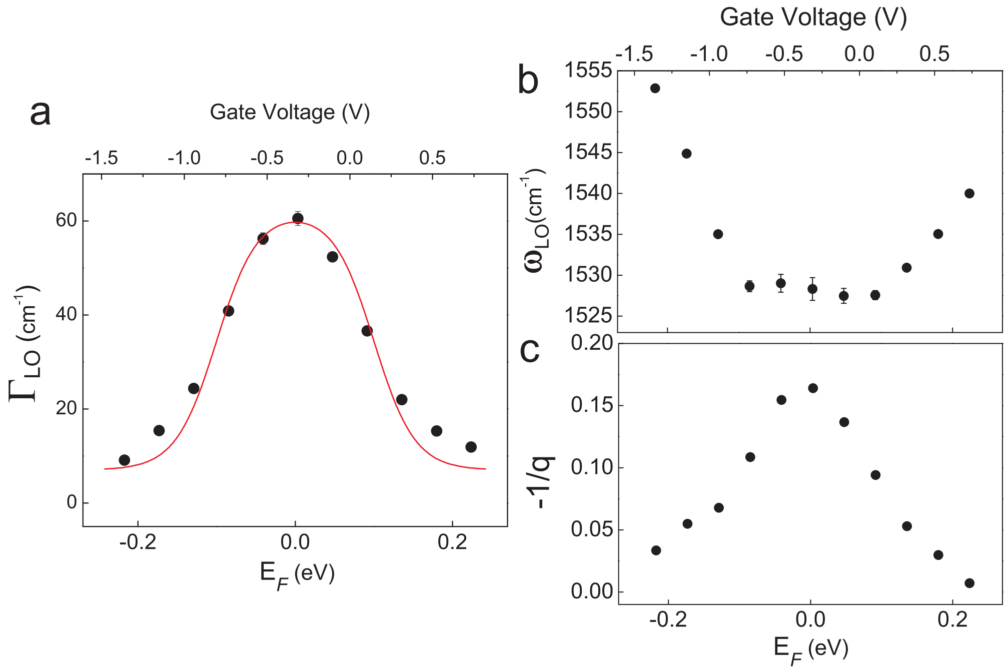


Fig. S 2: a) Linewidth $\Gamma_{LO}$ b) frequency $\omega_{LO}$ and c) asymmetry parameter $-1/q$ of the LO phonon peak as a function of gate voltage $V_g$ and Fermi energy.

$G^-$ peak is typically described by the Breit-Wigner-Fano lineshape

$$I_{LO}(\omega) = I_o \frac{[(q \cdot \Gamma_{LO} + (\omega - \omega_{LO}))]^2}{(\omega - \omega_{LO})^2 + \Gamma_{LO}^2}.$$

Here, $\omega_{LO}$ and $\Gamma_{LO}$ are the phonon frequency and linewidth, respectively, $I_o$ is a constant, and the Fano factor $1/q$ is a measure of the asymmetry of the Raman peak. The $G^-$ feature is fit to $I_{LO}(\omega) - I_o$, the isolated phonon contribution to the BWF lineshape.

Figure S2 shows the evolution of $\Gamma_{LO}$, $\omega_{LO}$ and $1/q$ as a function of the gate voltage $V_g$. The Fermi level scale on the bottom axes is related to $V_g$ by the linear relation $E_{\mathrm{F}}(V_g) = \alpha(V_g - V_o)$, where $\alpha = 0.21$ eV/V and $V_g = -0.33$ V are, respectively, the gate efficiency and charge neutrality voltage. This scaling is determined by fitting the broadening window in Fig. S2(a) to the function $\Gamma_{\mathrm{o}} + \Gamma_{\mathrm{ep}} f(T, E_{\mathrm{F}}, \hbar\omega_{LO})\,[1 + f(T, E_{\mathrm{F}}, -\hbar\omega_{LO})]$ [5, 12] which describes a window of width $\hbar\omega_{LO} \sim 0.2$ eV within which the LO phonon can create a real e-h excitation. The temperature, intrinsic linewidth, and electron-phonon linewidth are taken as $T = 300$ K, $\Gamma_{\mathrm{o}} = 7$ cm$^{-1}$ and $\Gamma_{\mathrm{ep}} = 55$ cm$^{-1}$, respectively. The same scaling of $E_{\mathrm{F}}(V_g)$ is used in Fig. 3. The narrowing in linewidth, upshift in frequency and decrease in asymmetry of the LO phonon feature as a function of $E_{\mathrm{F}}$ have been reported in a number

of recent works [5, 8, 10].


[1] R. Saito, G. Dresselhaus, and M. S. Dresselhaus, Phys. Rev. B **61**, 2981 (2000).

[2] M. Y. Sfeir *et al.*, Science **312**, 554 (2006).

[3] M. Y. Sfeir *et al.*, Science **306**, 1540 (2004).

[4] S. Berciaud *et al.*, Phys. Rev. B **81**, 041414(R) (2010).

[5] Y. Wu *et al.*, Phys. Rev. Lett. **99**, 027402 (2007).

[6] J. C. Meyer *et al.*, Phys. Rev. Lett. **95**, 217401 (2005).

[7] F. Wang *et al.*, Phys. Rev. Lett. **99**, (2007).

[8] H. Farhat *et al.*, Phys. Rev. Lett. **99**, 145506 (2007).

[9] A. Jorio, G. Dresselhaus, and M. S. Dresselhaus, *Carbon Nanotubes : Advanced Topics in the Synthesis, Structure, Properties and Applications* (Springer-Verlag, Berlin, 2008).

[10] J. C. Tsang *et al.*, Nano Nanotech. **2**, 725 (2007).

[11] S. Pisana *et al.*, Nature Mater. **6**, 198 (2007).

[12] N. Caudal, A. M. Saitta, M. Lazzeri, and F. Mauri, Phys. Rev. B **75**, 115423 (2007).
